# Supplementary material for: Fully Dynamic Effective Resistances
Source: arXiv:1804.04038 source file (2018-04-11)
Supplement: Supplementary file 1 [file properties_random_walks_appendix.tex]

%We provide a bit more details on the behavior of
%random walks used in proving the congestion of edges
%in Corollary~\ref{cor:Load}.
%By symmetry, we can fix the edge in question as
%\[
%\ehat
%=
%\uhat \vhat,
%\]
%and without loss of generality consider only the probability
%of a walk reaching $\ehat$ via the vertex $\uhat$.
%
%Then we define the random variable
%\[
%X_{\uhat, u, i}
%\]
%as the probability that a random walk starting at $u$
%passes through the vertex $\uhat$ after $i$ steps.
%
%The invocation of Chernoff bounds in the proof of
%Corollary~\ref{cor:Load} is working with the quantities
%\[
%X_{u}
%=
%\frac{1}{\deg\left( \uhat \right)}
%\sum_{0 \leq t \leq L}
%\deg\left( u \right)
%\cdot
%X_{\uhat, u, t}.
%\]
%for some length $L$.
%Note that the number of walks starting at $u$ is $\deg(u)$
%because we're starting one random walk per end point of each edge.
%
%First, note that because the walks are independent,
%the quantities $X_{u}$ are also independent.
%Note however $X_{\ehat, u, t_1}$ and $X_{\ehat, e, t_2}$
%are not independent: the walk's
%$(t+1)\textsuperscript{th}$ location depends
%on its $t\textsuperscript{th}$ location.
%Thus, we can only use the bound
%\[
%X_{u} \leq L
%\]
%obtained from $X_{\uhat, u, i} \leq 1$.
%In fact, this bound is tight up to constants:
%consider random walking on a graph with a
%single edge $e = uv$, and $\uhat = u$.
%
%Our key bound is showing that
%\[
%\frac{1}{\deg\left( \uhat \right)}
%\sum_{u} \expec{}{X_u}
%=
%\frac{1}{\deg\left( \uhat \right)}
%\sum_{u \in V, 0 \leq t \leq L}
%\deg\left( u \right) X_{\ehat, e, t}
%\]
%can also be bounded by $L$.



%
%
%The following lemmas then bound how many walks need to be regenerated. \todo{Encompass them into one main lemma}
%\begin{definition}
%	Let $\walk{t}{v}$ be an $t$-step random walk starting at $v$. Then for each vertex, we will take $\kappa \deg(v)$ random $t$-step walks, for some $\kappa$, and let \[\walks{t}{G}{\kappa} = \bigcup_{v\in V} \kappa \deg(v) \walk{t}{v} \]
%	
%	Note that the number of walks in $\walks{t}{G}{\kappa}$ is $2\kappa m$.
%	
%\end{definition}
%\begin{lemma}\label{lem:randomWalkInvariant} For any graph $G$ and vertex $v$
%	\[
%	\expec{}{\text{number of $\walks{t}{G}{\kappa}$ that end at v}} = \kappa\deg(v)
%	\]
%\end{lemma}
%
%\begin{proof}
%	By induction. True by definition for $t = 0$. Further,
%	
%	\[
%	\expec{}{\text{number of $\walks{t}{G}{\kappa}$ that end at v}} = \sum_{u \sim v} \expec{}{\text{number of $\walks{t-1}{G}{\kappa}$ that end at u}} \frac{1}{\deg(u)}
%	\]
%	
%	and applying our inductive hypothesis implies the claim.
%\end{proof}
%
%\begin{lemma}
%\label{lem:randomWalkEdge}
%	For any graph $G$ and edge $e = (u,v)$, 
%	
%	\[
%	\expec{}{\text{number of $\walks{t}{G}{\kappa}$ that use $e$}} \leq 2\kappa \cdot t
%	\]
%	
%\end{lemma}
%
%\begin{proof}
%	\begin{multline*}
%	\expec{}{\text{number of $\walks{t}{G}{\kappa}$ that use $e$}} \leq \\ \sum_{i=1}^l \expec{}{\text{number of $\walks{t}{G}{\kappa}$ that use $e$ on $i$th step}} 
%	\end{multline*}
%	
%	In order to use $e$ on the $i$th step, the walk must have been at either $u$ or $v$ on the $(i-1)$th step. Therefore
%	
%	\begin{multline*}
%	\expec{}{\text{number of $\walks{t}{G}{\kappa}$ that use $e$ on $i$th step}} = \\ 
%	\expec{}{\text{number of $\walks{i-1}{G}{\kappa}$ that end at v}} \frac{1}{\deg(v)} + \\
%	\expec{}{\text{number of $\walks{i-1}{G}{\kappa}$ that end at u}} \frac{1}{\deg(u)}
%	\end{multline*}
%	Applying Lemma~\ref{lem:randomWalkInvariant} reduces this to 4, and implies our desired result.
%\end{proof}
%
%\begin{lemma}
%	For any graph $G$ and edge $e = uv$, 
%	
%	\[
%	\expec{}{\text{number of occurences in $\walks{t}{G}{\kappa}$ of vertex $v$}} \leq \deg(v) \kappa\cdot t
%	\]
%	
%\end{lemma}
%
%\begin{proof}
%	\begin{multline*}
%	\expec{}{\text{number of occurences in $\walks{t}{G}{\kappa}$ of vertex $v$}} = \\
%	\sum_{i=1}^l \expec{}{\text{number of $\walks{i}{G}{\kappa}$ end at vertex $v$}}
%	\end{multline*}
%	
%	Then just apply Lemma~\ref{lem:randomWalkInvariant}.
%	
%\end{proof}
